# Supplementary material for: The Llama 3 Herd of Models
Source: arXiv:2407.21783 source file (2024-11-23)
Supplement: Supplementary file 7 [file speech_appendix.tex]

\section{Speech Evaluation Results}
\label{section:speechappendix}
In this section, we present the non-aggregated results on the multilingual benchmarks.
Table~\ref{tab:sphapp:fleursasr} reports the FLEURS speech recognition.
Table~\ref{tab:sphapp:fleursast} reports the FLEURS speech translation.
Table~\ref{tab:sphapp:cvst2ast} reports the Covost 2 speech translation.
The reported numbers from Whisper and SeamlessM4T are included as reference.

\begin{table}
	\centering
	\begin{NiceTabular}{lcccc}
	\CodeBefore
	\Body
	\toprule
	Language &  Llama 3 8B & Llama 3 70B & Whisper v3 & SeamlessM4T v2 \\
	\midrule
	Italian	&	3.7	&	3.3	&	3.0	&	6.1	\\
	Spanish	&	3.8	&	3.1	&	2.8	&	6.6	\\
	Korean	&	4.8	&	3.7	&	3.1	&	7.2	\\
	English	&	5.7	&	4.5	&	4.1	&	7.4	\\
	Portuguese	&	5.7	&	4.5	&	4.1	&	9.2	\\
	Indonesian	&	5.8	&	5.0	&	6.1	&	9.5	\\
	French	&	6.3	&	5.6	&	5.3	&	8.4	\\
	German	&	6.5	&	5.7	&	4.9	&	8.2	\\
	Japanese	&	7.2	&	7.2	&	4.9	&	12.1	\\
	Hindi	&	7.8	&	6.1	&	17.0	&	11.0	\\
	Kannada	&	7.9	&	7.2	&	33.0	&	14.4	\\
	Russian	&	7.9	&	6.9	&	5.0	&	10.3	\\
	Dutch	&	7.9	&	6.6	&	5.2	&	9.7	\\
	Polish	&	8.4	&	6.6	&	4.6	&	10.2	\\
	Bengali	&	8.7	&	7.6	&	50.0	&	8.6	\\
	Vietnamese	&	8.8	&	7.4	&	8.6	&	9.9	\\
	Malayalam	&	8.9	&	7.9	&	--	&	12.8	\\
	Thai	&	9.0	&	7.7	&	8.4	&	11.3	\\
	Chinese	&	9.1	&	7.8	&	7.7	&	11.4	\\
	Gujarati	&	9.8	&	9.2	&	47.4	&	13.4	\\
	Marathi	&	10.1	&	8.3	&	34.1	&	13.9	\\
	Turkish	&	10.4	&	8.3	&	6.7	&	12.3	\\
	Tamil	&	10.7	&	10.5	&	18.3	&	15.0	\\
	Finnish	&	10.9	&	8.3	&	7.7	&	14.0	\\
	Romanian	&	11.3	&	8.4	&	8.2	&	11.0	\\
	Swedish	&	12.0	&	9.6	&	7.6	&	12.8	\\
	Czech	&	12.5	&	9.8	&	10.1	&	11.9	\\
	Persian	&	12.6	&	12.7	&	29.4	&	23.5	\\
	Swahili	&	12.8	&	12.7	&	34.1	&	15.0	\\
	Telugu	&	13.2	&	12.3	&	39.3	&	15.9	\\
	Greek	&	13.8	&	11.9	&	10.9	&	11.2	\\
	Arabic	&	14.0	&	13.0	&	9.6	&	14.8	\\
	Hungarian	&	18.6	&	11.8	&	12.9	&	13.9	\\
	Urdu	&	19.0	&	17.2	&	20.6	&	17.5	\\
	\midrule
	Average &9.6 & 8.2 &	14.4	&	11.8	 \\
	\bottomrule
\end{NiceTabular}

	\caption{Non-aggregated evaluation results on FLEURS speech recognition (metric: word error rate \%).}
	\label{tab:sphapp:fleursasr}
\end{table}

\begin{table}
	\centering
	\begin{NiceTabular}{lcccc}
	\CodeBefore
	\Body
	\toprule
	X$\rightarrow$English & Llama 3 8B & Llama 3 70B & Whisper v2 & SeamlessM4T v2 \\
	\midrule
	Portuguese	&	44.4	&	48.4	&	38.1	&	38.4	\\
	German	&	40.2	&	42.7	&	34.6	&	37.0	\\
	French	&	40.0	&	42.2	&	32.2	&	34.0	\\
	Swedish	&	37.6	&	43.2	&	35.3	&	36.9	\\
	Romanian	&	36.9	&	41.0	&	31.5	&	35.0	\\
	Indonesian	&	36.6	&	42.9	&	29.1	&	32.7	\\
	Arabic	&	36.0	&	40.9	&	25.5	&	34.6	\\
	Russian	&	33.0	&	36.9	&	27.8	&	30.2	\\
	Czech	&	32.9	&	37.4	&	27.8	&	34.0	\\
	Italian	&	31.9	&	34.6	&	23.6	&	26.5	\\
	Spanish	&	31.8	&	34.4	&	23.3	&	25.5	\\
	Swahili	&	31.4	&	37.9	&	7.2	&	31.1	\\
	Dutch	&	31.0	&	32.1	&	24.0	&	27.8	\\
	Persian	&	30.5	&	34.8	&	19.6	&	30.3	\\
	Finnish	&	29.6	&	34.5	&	22.1	&	28.0	\\
	Greek	&	28.7	&	31.6	&	23.7	&	27.1	\\
	Hindi	&	28.4	&	35.0	&	22.0	&	28.2	\\
	Turkish	&	28.3	&	36.9	&	26.6	&	30.7	\\
	Gujarati	&	27.8	&	33.3	&	16.2	&	31.4	\\
	Polish	&	26.4	&	29.1	&	22.3	&	24.4	\\
	Hungarian	&	26.3	&	32.3	&	21.2	&	27.8	\\
	Bengali	&	26.1	&	30.2	&	13.2	&	26.3	\\
	Malayalam	&	25.4	&	29.7	&	16.7	&	26.0	\\
	Urdu	&	25.3	&	30.0	&	17.2	&	24.4	\\
	Vietnamese	&	24.7	&	27.6	&	20.4	&	26.0	\\
	Kannada	&	24.7	&	28.8	&	11.6	&	25.1	\\
	Thai	&	23.7	&	26.9	&	16.1	&	23.2	\\
	Marathi	&	23.5	&	29.5	&	12.9	&	27.4	\\
	Telugu	&	23.5	&	25.0	&	12.5	&	25.1	\\
	Chinese	&	23.4	&	25.7	&	18.4	&	23.0	\\
	Korean	&	21.7	&	25.9	&	21.3	&	24.1	\\
	Japanese	&	21.0	&	25.3	&	18.9	&	18.2	\\
	Tamil	&	20.9	&	24.7	&	9.2	&	22.2	\\
	\midrule
	Average & 29.5 & 33.7 & 21.9 & 28.6 \\
	\bottomrule
\end{NiceTabular}

	\caption{Non-aggregated evaluation results on FLEURS speech translation (metric: BLEU score).}
	\label{tab:sphapp:fleursast}
\end{table}

\begin{table}
	\centering
	\begin{NiceTabular}{lcccc}
	\CodeBefore
	\Body
	\toprule
	X$\rightarrow$English & Llama 3 8B & Llama 3 70B & Whisper v2 & SeamlessM4T v2 \\
	\midrule
	Portuguese	&	48.4	&	55.1	&	51.6	&	53.8	\\
	Indonesian	&	47.9	&	51.1	&	48.1	&	52.4	\\
	Arabic	&	45.5	&	48.6	&	39.7	&	46.7	\\
	Russian	&	43.9	&	50.3	&	43.3	&	53.6	\\
	Dutch	&	42.3	&	45.5	&	41.2	&	42.8	\\
	French	&	40.6	&	43.5	&	36.4	&	42.1	\\
	Spanish	&	40.2	&	43.8	&	40.1	&	42.9	\\
	German	&	38.0	&	42.0	&	36.3	&	39.9	\\
	Italian	&	37.3	&	41.1	&	30.9	&	40.0	\\
	Swedish	&	36.0	&	44.8	&	42.9	&	43.5	\\
	Turkish	&	28.8	&	31.8	&	28.3	&	33.1	\\
	Persian	&	24.7	&	26.6	&	19.3	&	27.2	\\
	Japanese	&	24.5	&	28.3	&	26.1	&	23.8	\\
	Chinese	&	15.2	&	23.8	&	18.0	&	22.2	\\
	Tamil	&	2.2	&	6.0	&	4.2	&	4.6	\\
	\midrule
	Average & 34.4& 38.8 & 33.8 & 37.9 \\
	\bottomrule
\end{NiceTabular}

	\caption{Non-aggregated evaluation results on Covost 2 speech translation (metric: BLEU score).}
	\label{tab:sphapp:cvst2ast}
\end{table}
